# Supplementary material for: Solving integral equations in $\eta\to 3\pi$
Source: arXiv:1809.06399 ancillary file (2018-12-13)
Supplement: Supplementary file 1 [file READMEv2.pdf]

# Fundamental solutions: Notation, Input, Update

J. Gasser<sup>1</sup> and A. Rusetsky<sup>2</sup>

## Contents

|                     |                                                                                                             |                    |
|---------------------|-------------------------------------------------------------------------------------------------------------|--------------------|
| <a href="#">1</a>   | <a href="#">The files</a>                                                                                   | <a href="#">1</a>  |
| <a href="#">2</a>   | <a href="#">The integral equations</a>                                                                      | <a href="#">2</a>  |
| <a href="#">3</a>   | <a href="#">Fundamental solutions</a>                                                                       | <a href="#">3</a>  |
| <a href="#">4</a>   | <a href="#">Phase shifts</a>                                                                                | <a href="#">3</a>  |
| <a href="#">5</a>   | <a href="#">The 8 sets of phase shifts used as input</a>                                                    | <a href="#">4</a>  |
| <a href="#">6</a>   | <a href="#">Numerical constants and dimensions</a>                                                          | <a href="#">5</a>  |
| <a href="#">7</a>   | <a href="#">The fundamental solutions</a>                                                                   | <a href="#">6</a>  |
| <a href="#">8</a>   | <a href="#">Update</a>                                                                                      | <a href="#">6</a>  |
| <a href="#">8.1</a> | <a href="#">Spikes . . . . .</a>                                                                            | <a href="#">6</a>  |
| <a href="#">8.2</a> | <a href="#">Reasons for the occurrence of spikes . . . . .</a>                                              | <a href="#">7</a>  |
| <a href="#">8.3</a> | <a href="#">Check absence of spikes . . . . .</a>                                                           | <a href="#">8</a>  |
| <a href="#">8.4</a> | <a href="#">Updated solutions . . . . .</a>                                                                 | <a href="#">8</a>  |
| <a href="#">8.5</a> | <a href="#">Implication for the numerical analysis of <math>\eta \rightarrow 3\pi</math> decays . . . .</a> | <a href="#">10</a> |

## 1 The files

In the following, we recall the integral equations solved and describe the content of the files

MI\_S\_P\_v2.dat    fundamental solutions

---

<sup>1</sup>gasser@itp.unibe.ch

<sup>2</sup>rusetsky@hiskp.uni-bonn.de

$$\left. \begin{array}{l} \text{TS\_P.dat} \\ \text{phases\_P.dat} \end{array} \right\} \text{ phase shifts used}$$

Furthermore, we comment on the difference between the updated solutions `MI_S_P_v2.dat` and the former ones, `MI_S_P.dat`.

## 2 The integral equations

We use the conventions of Ref. [1]. The integral equations read

$$\begin{aligned} M_0(s) &= \Omega_0(s) \left\{ \alpha_0 + \beta_0 s + \gamma_0 s^2 + \delta_0 s^3 + s^2 \int_{4M_\pi^2}^{\infty} d\mu_0(s') \frac{\hat{M}_0(s')}{s' - s - i\varepsilon} \right\}, \\ M_1(s) &= \Omega_1(s) \left\{ \beta_1 s + \gamma_1 s^2 + s \int_{4M_\pi^2}^{\infty} d\mu_1(s') \frac{s' \hat{M}_1(s')}{s' - s - i\varepsilon} \right\}, \\ M_2(s) &= \Omega_2(s) s^2 \int_{4M_\pi^2}^{\infty} d\mu_2(s') \frac{\hat{M}_2(s')}{s' - s - i\varepsilon}. \end{aligned} \quad (1)$$

Here, the integration measure is

$$d\mu_I(s') = \frac{ds'}{\pi s'^2} \frac{\sin \delta_I(s')}{|\Omega_I(s')|}, \quad (2)$$

and the “hat” functions are given by

$$\begin{aligned} \hat{M}_0 &= \frac{2}{3} \langle M_0 \rangle + 2(s - s_0) \langle M_1 \rangle + \frac{2}{3} \kappa \langle z M_1 \rangle + \frac{20}{9} \langle M_2 \rangle, \\ \hat{M}_1 &= \kappa^{-1} \left\{ 3 \langle z M_0 \rangle + \frac{9}{2} (s - s_0) \langle z M_1 \rangle - 5 \langle z M_2 \rangle + \frac{3}{2} \kappa \langle z^2 M_1 \rangle \right\}, \\ \hat{M}_2 &= \langle M_0 \rangle - \frac{3}{2} (s - s_0) \langle M_1 \rangle - \frac{1}{2} \kappa \langle z M_1 \rangle + \frac{1}{3} \langle z M_2 \rangle. \end{aligned} \quad (3)$$

Here,  $\hat{M}_I = \hat{M}_I(s)$ ,  $\langle z^m M_I \rangle = \langle z^m M_I \rangle(s)$ , and

$$\begin{aligned} s_0 &= \frac{1}{3} M_\eta^2 + M_\pi^2, \\ \kappa(s) &= \sqrt{1 - \frac{4M_\pi^2}{s}} \sqrt{(M_\eta - M_\pi)^2 - s} \sqrt{(M_\eta + M_\pi)^2 - s}. \end{aligned} \quad (4)$$

The angular averages are defined as

$$\langle z^n M_I \rangle(s) = \frac{1}{2} \int_{-1}^1 dz z^n M_I \left( \frac{3}{2} s_0 - \frac{1}{2} s + \frac{1}{2} z \kappa(s) \right). \quad (5)$$

The Omnès functions are expressed through the S-wave phase shifts with isospin  $I = 0, 2$  and the P-wave phase shift with isospin  $I = 1$ :

$$\Omega_I(s) = \exp \left\{ \frac{s}{\pi} \int_{4M_\pi^2}^{\infty} \frac{ds'}{s'} \frac{\delta_I(s')}{s' - s - i\varepsilon} \right\}. \quad (6)$$

The relation to the standard notation is  $\delta_0 = \delta_0^0, \delta_2 = \delta_0^2, \delta_1 = \delta_1^1$ .

### 3 Fundamental solutions

The general solution of the system of integral equations (1) is given as a linear combination of six fundamental solutions:

$$M_I(s) = \alpha_0 M_I^{\alpha_0}(s) + \beta_0 M_I^{\beta_0}(s) + \cdots + \gamma_1 M_I^{\gamma_1}(s). \quad (7)$$

Here,  $M_I^{\alpha_0}(s)$  is the solution with  $\alpha_0 = 1, \beta_0 = \gamma_0 = \delta_0 = \beta_1 = \gamma_1 = 0$ , etc.

The fundamental solutions are uniquely determined by the  $\pi\pi$  phase shifts [1]. In the following, we tabulate the fundamental solutions for 8 different sets of phase shifts, in the energy range

$$0.02125 M_\pi^2 \leq s \leq 19.9575 M_\pi^2. \quad (8)$$

We now describe the phase shifts used.

### 4 Phase shifts

$$\underline{2M_\pi \leq E \leq 0.8 \text{ GeV}}$$

Below the CM energy of two pions  $E = \sqrt{s} \leq 0.8 \text{ GeV}$ , we use the representation given in Refs. [2, 3],

$$\tan \delta_I(s) = \sqrt{1 - \frac{4M_\pi^2}{s}} q^{2\ell} (A_{\ell I} + B_{\ell I} q^2 + C_{\ell I} q^4 + D_{\ell I} q^6) \frac{4M_\pi^2 - s_{\ell I}}{s - s_{\ell I}}. \quad (9)$$

Here, the total angular momentum is  $\ell = 0$  for  $I = 0, 2$  and  $\ell = 1$  for  $I = 1$ . Further,

$$q^2 = \frac{s}{4} - M_\pi^2. \quad (10)$$

For a given set of phase shifts, one needs 15 Schenk parameters  $A_{00}, \dots, s_{02}$ .

$0.8 \leq E \leq 1.7$  GeV

We use tables for  $\delta_{0,1,2}$  at discrete values of the CM energy  $E$ . These tables were provided to us by the authors of Ref. [1].

$E \geq 1.7$  GeV

Here, we set

$$\delta_0 = \delta_1 = \pi, \delta_2 = 0. \quad (11)$$

As a result of this choice, the integrations in (1) are chopped off at  $s' = (1.7\text{GeV})^2$ . At  $E = 0.8$  GeV and at  $E = 1.7$  GeV, the phase shifts are glued together in a continuous manner.

## 5 The 8 sets of phase shifts used as input

In order to provide a solid basis for the evaluation of uncertainties in the analysis of  $\eta \rightarrow 3\pi$ , we have determined the fundamental solutions for 8 sets of phase shifts. A given set of phase shifts is characterized by its Schenk parameters and by the phase shifts between 0.8 GeV and 1.7 GeV. The data is provided in 2 tables,

|                           |                                   |
|---------------------------|-----------------------------------|
| <code>TS_P.dat</code>     | Schenk parameters                 |
| <code>phases_P.dat</code> | phase shifts; $P = 0, \dots, 7$ . |

- The Schenk parameters in `TS_P.dat` are tabulated in the following order (in GeV units),

$A_{00}$   
 $B_{00}$   
 $C_{00}$   
 $D_{00}$   
 $S_{00}$   
 $A_{11}$   
 $\vdots$   
 $S_{11}$   
 $A_{02}$   
 $\vdots$   
 $S_{02}$

- The phase shifts in `phases_P.dat` are presented in 4 columns,

CM energy  $E$  (in GeV) |  $\delta_0$  |  $\delta_1$  |  $\delta_2$  (in degrees)

The first 7 sets are distinguished by the value of the phase shifts at  $s=(0.8 \text{ GeV})^2$ ,

| $\bar{\delta}_0$ | $\bar{\delta}_1$ | $\bar{\delta}_2$ | P |
|------------------|------------------|------------------|---|
| 82.3             | 108.9            | -19.5            | 0 |
| 92.3             | 108.9            | -19.5            | 1 |
| 78.3             | 108.9            | -19.5            | 2 |
| 82.3             | 110.9            | -19.5            | 3 |
| 82.3             | 106.9            | -19.5            | 4 |
| 82.3             | 108.9            | -18.7            | 5 |
| 82.3             | 108.9            | -20.0            | 6 |

with  $\bar{\delta}_I = \delta_I(s = (0.8\text{GeV})^2)$ . In the set  $P = 7$ , the  $I = 0$  S-wave is set to  $\delta_0 \sim \pi$  above 1 GeV, the two other phases are kept at the value of the set with  $P = 0$ .

The set  $P = 0$  corresponds to the central values of the input. The other sets may be used to estimate systematic uncertainties.

## 6 Numerical constants and dimensions

We use

$$M_\pi = .13957018 \text{ GeV}, \quad M_\eta = .547853 \text{ GeV}. \quad (12)$$

The amplitudes  $M_I$  and  $M_I^{\alpha_0, \beta_0, \dots, \gamma_1}$  with  $I = 0, 2$  ( $I = 1$ ) are dimensionless (carry dimension  $\text{mass}^{-2}$ ). Dimensionful quantities are given in units of GeV.

## 7 The fundamental solutions

Our results for the fundamental solutions are contained in the files `MI_S_P_v2.dat`, where

- $I = 0, 1, 2$  : Labels the isospin
- $S = 1, \dots, 6$  : Labels the fundamental solution:  
 $S = 1 \rightarrow \alpha_0 = 1, S = 2 \rightarrow \beta_0 = 1, \dots, S = 6 \rightarrow \gamma_1 = 1$
- $P = 0, \dots, 7$  : Labels the  $\pi\pi$  phase shifts used.

The three columns in the table `MI_S_P_v2.dat` contain the values of  $s/M_\pi^2$  and the real and imaginary parts of the fundamental solution  $S$  with isospin  $I$ , evaluated with phase shifts  $P$ . To wit, the fifth line in `M1_2_3_v2.dat` reads

0.116250000000000002 1.97667842984088570E-004 5.72717437224096472E-005

and signifies that

$$\begin{aligned}
 sM_\pi^{-2} &= 0.116250000000000002, \\
 \text{Real part} &= 1.97667842984088570 \cdot 10^{-4} \text{GeV}^{-2}, \\
 \text{Imag. part} &= 5.72717437224096472 \cdot 10^{-5} \text{GeV}^{-2}
 \end{aligned} \tag{13}$$

for the fundamental solution  $M_1^{\beta_0}$ , evaluated with the set of phase shifts  $P = 3$ .

## 8 Update

### 8.1 Spikes

As Bachir Moussallam pointed out to us [4], tiny spikes occur in our former fundamental solutions `MI_S_P` [5, version v1], see Fig. 1 for the case of `M0_1_0`. Note that the spike is so small that it is not visible on a reasonable scale.

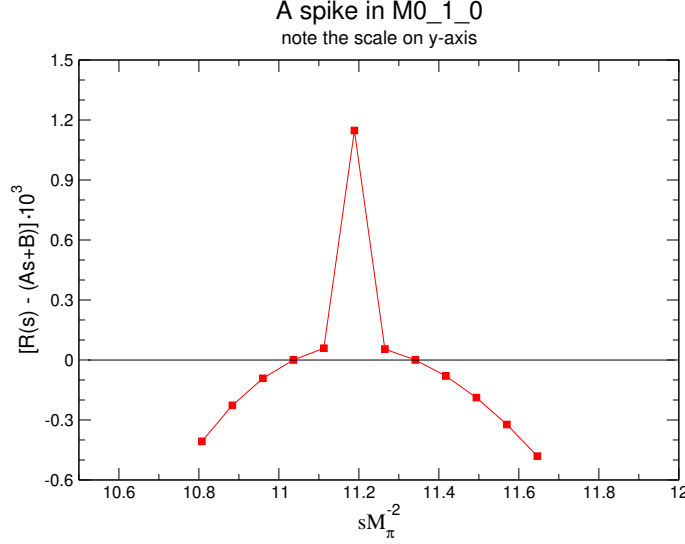

Figure 1: A spike in the fundamental solution M0\_1\_0 at  $s = 11.1888M_\pi^2$ . Notation:  $R(s)$  denotes the real part of M0\_1\_0, and  $As + B$  goes through  $R(s)$  at  $s_1 = 11.0363M_\pi^2$  and at  $s_2 = 11.3412M_\pi^2$ . Displayed is the difference  $[R(s) - (As + B)] \cdot 10^3$ . The horizontal line at  $y = 0$  is set to guide the eye. The figure is similar to the one sent to us by Moussallam [4]. See text for more details.

## 8.2 Reasons for the occurrence of spikes

There are two reasons for the occurrence of spikes:

- Principal value integrals for the Omnès function were performed in [5] with a commercial Fortran routine, which then generated spikes like the one displayed in Fig. 1. We have now replaced that routine by using

$$\oint_A^B \frac{f(x) dx}{x-s} = f(s) \oint_A^B \frac{dx}{x-s} + \int_A^B \frac{[f(x) - f(s)] dx}{x-s}; \quad s \in (A, B), (14)$$

where  $\oint$  denotes a principal value integral. The first integral on the right-hand side is performed analytically, the second, an ordinary one, numerically.

- Very near the threshold  $s = 4M_\pi^2$ , a second type of (tiny) spikes may occur. They are generated by an integrable square-root singularity that

we now tame by performing a transformation of variable,

$$z = A + (B - A) \tau^2, 0 \leq \tau \leq 1, \quad (15)$$

see [5, section 5].

### 8.3 Check absence of spikes

We have generated updates of the 144 fundamental solutions using (14,15). How can one make sure that there are no spikes left somewhere? As these spikes are on a very small scale, a visual detection in a figure is impossible. It would therefore be nice to have a numerical test that would automatically confirm the absence/presence of spikes. We did not find such an automatic test. Instead, we proceed as follows. Whenever there is a spike at  $s = s_0$ , the derivative of the solution will fluctuate around the point  $s_0$ . Moreover, the second derivative will fluctuate even more violently. So, the check consists in evaluating the first and second derivatives, approximated by

$$\begin{aligned} f'(s_j) &= \frac{M_\pi^2 [f(s_j) - f(s_{j-1})]}{s_j - s_{j-1}}, \\ f''(s_j) &= \frac{M_\pi^2 [f'(s_j) - f'(s_{j-1})]}{s_j - s_{j-1}}, \end{aligned} \quad (16)$$

where  $f(s_j)$  denotes the real or imaginary part of a fundamental solution. Then we check visually whether a spike is present. This is possible, because the spikes in the derivatives are rather big. As an illustration, we display in Fig. 2 the first derivative of the real part of M0\_1\_0 and of an update, where the principal value integral was performed with (14). The derivative is displayed around  $s = 11.2M_\pi^2$ , where the spike in Fig. 1 occurs. We display the first derivative of the original solution, and of the update. The improvement in the behaviour of  $f(s)$  is clearly seen.

### 8.4 Updated solutions

In table 1, we display the relative changes in the fundamental solutions for the central values of the phase shifts ( $P = 0$ ),

$$\text{delta}_I = \max_{\{S\}} \left| \frac{\text{MI\_S\_0}}{\text{MI\_S\_0\_v2}} - 1 \right|, \quad (17)$$



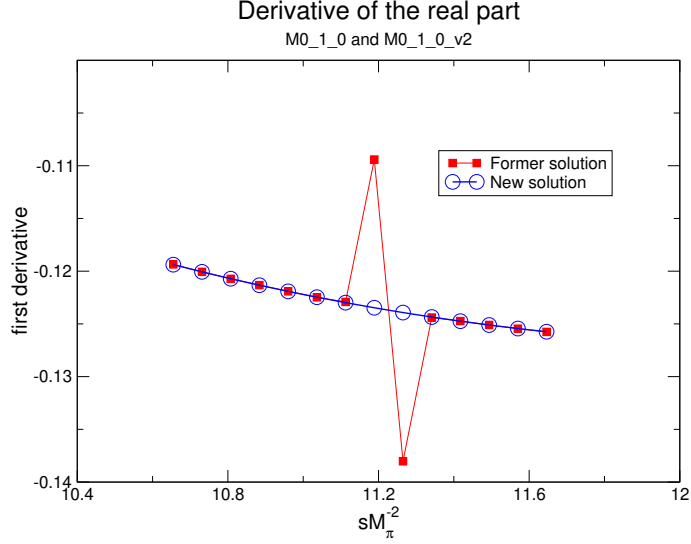

Figure 2: First derivative of the real part of  $M0\_1\_0$  and of its update around  $s = 11.2M_\pi^2$ . Red: Original solution. Blue: updated solution, done with (14).

where the maximum is taken over the pertinent region,

$$\begin{aligned}
\text{region 1:} & \quad 0.045M_\pi^2 < s < 4M_\pi^2, \\
\text{region 2:} & \quad s = 4M_\pi^2, \\
\text{region 3:} & \quad 4M_\pi^2 < s < (M_\eta - M_\pi)^2, \\
\text{region 4:} & \quad (M_\eta - M_\pi)^2 < s < 19.958M_\pi^2,
\end{aligned} \tag{18}$$

and over the fundamental solutions  $S = 1, \dots, 6$ . For example, the maximal relative change in the region  $0.045M_\pi^2 < s < 4M_\pi^2$  for isospin 1 is  $\delta a_1 = 1.4 \cdot 10^{-6}$ .

In table 2, we display the relative changes

$$\text{DELTA}_I = \max_{\{S,P\}} \left| \frac{\text{MI\_S\_P}}{\text{MI\_S\_P\_v2}} - 1 \right|, \tag{19}$$

where the maximum is taken over the pertinent region, over the fundamental solutions  $S = 1, \dots, 6$  and over all phases  $P = 0, \dots, 7$ .

| isospin | region 1            | region 2            | region 3            | region 4            |
|---------|---------------------|---------------------|---------------------|---------------------|
| 0       | $2.4 \cdot 10^{-4}$ | $3.6 \cdot 10^{-3}$ | $7.1 \cdot 10^{-4}$ | $9.0 \cdot 10^{-4}$ |
| 1       | $1.4 \cdot 10^{-6}$ | $1.6 \cdot 10^{-6}$ | $1.3 \cdot 10^{-5}$ | $1.4 \cdot 10^{-4}$ |
| 2       | $7.6 \cdot 10^{-4}$ | $1.1 \cdot 10^{-2}$ | $2.0 \cdot 10^{-3}$ | $3.8 \cdot 10^{-4}$ |

Table 1: Relative changes  $\delta_I$ , see Eq. (17).

| isospin | region 1            | region 2            | region 3            | region 4            |
|---------|---------------------|---------------------|---------------------|---------------------|
| 0       | $1.2 \cdot 10^{-3}$ | $1.6 \cdot 10^{-2}$ | $3.1 \cdot 10^{-3}$ | $9.0 \cdot 10^{-4}$ |
| 1       | $1.5 \cdot 10^{-6}$ | $1.9 \cdot 10^{-6}$ | $3.0 \cdot 10^{-4}$ | $1.3 \cdot 10^{-3}$ |
| 2       | $9.3 \cdot 10^{-4}$ | $1.3 \cdot 10^{-2}$ | $2.4 \cdot 10^{-3}$ | $2.1 \cdot 10^{-3}$ |

Table 2: Relative changes  $\Delta_I$ , see Eq. (19).

## 8.5 Implication for the numerical analysis of $\eta \rightarrow 3\pi$ decays

We emphasize that the numerical effects discussed above are too small to significantly affect the results obtained for the various physical quantities in [1]. These are based on the old numerical tables for the fundamental solutions [5, version v1]. To illustrate the difference between the old and new solutions, we consider the quark mass ratio  $Q$ , for which the final results of [1] are quoted in equation (9.18):  $Q = 22.04(72)$  and  $Q = 22.08(66)$  for the charged and neutral channels, respectively. At this accuracy, repeating the calculation with the new basis leads to the same outcome for  $Q$  [6]. The difference only shows up in the fifth or sixth decimal: in the charged channel the value 22.041666 (old) is shifted to 22.041660 (new), while in the neutral channel, the corresponding numbers are 22.083670 (old) and 22.083622 (new). This shows that the errors in the result for  $Q$  generated by the shortcomings

of the old representation are smaller than the quoted uncertainties by about four orders of magnitude.

## Acknowledgments

We thank Bachir Moussallam for pointing out to us the presence of spikes in the old fundamental solutions, and Heinrich Leutwyler for verification that the changes in the fundamental solutions – generated by the elimination of the spikes – are too small to significantly affect the results obtained for the various physical quantities in [1].

## References

- [1] G. Colangelo, S. Lanz, H. Leutwyler and E. Passemar, *Dispersive analysis of  $\eta \rightarrow 3\pi$* , *Eur. Phys. J.* **C78** (2018) 947 [[arXiv:1807.11937](#)].
- [2] A. Schenk, *Absorption and dispersion of pions at finite temperature*, *Nucl. Phys.* **B363** (1991) 97.
- [3] G. Colangelo, J. Gasser and H. Leutwyler,  *$\pi\pi$  scattering*, *Nucl. Phys.* **B603** (2001) 125 [[hep-ph/0103088](#)].
- [4] B. Moussallam, private communication.
- [5] J. Gasser and A. Rusetsky, *Solving integral equations in  $\eta \rightarrow 3\pi$* , *Eur. Phys. J.* **C78** (2018) 906 [[arXiv:1809.06399](#)].
- [6] H. Leutwyler, private communication.
